# Supplementary material for: Map-based cosmology inference with lognormal cosmic shear maps
Source: arXiv:2204.13216 source file (2022-04-27)
Supplement: Supplementary file 1 [file emulator.tex]

\section{Emulator accuracy}\label{sec:emulator}

% \begin{figure*}
%     \centering
%     \includegraphics[width=\linewidth]{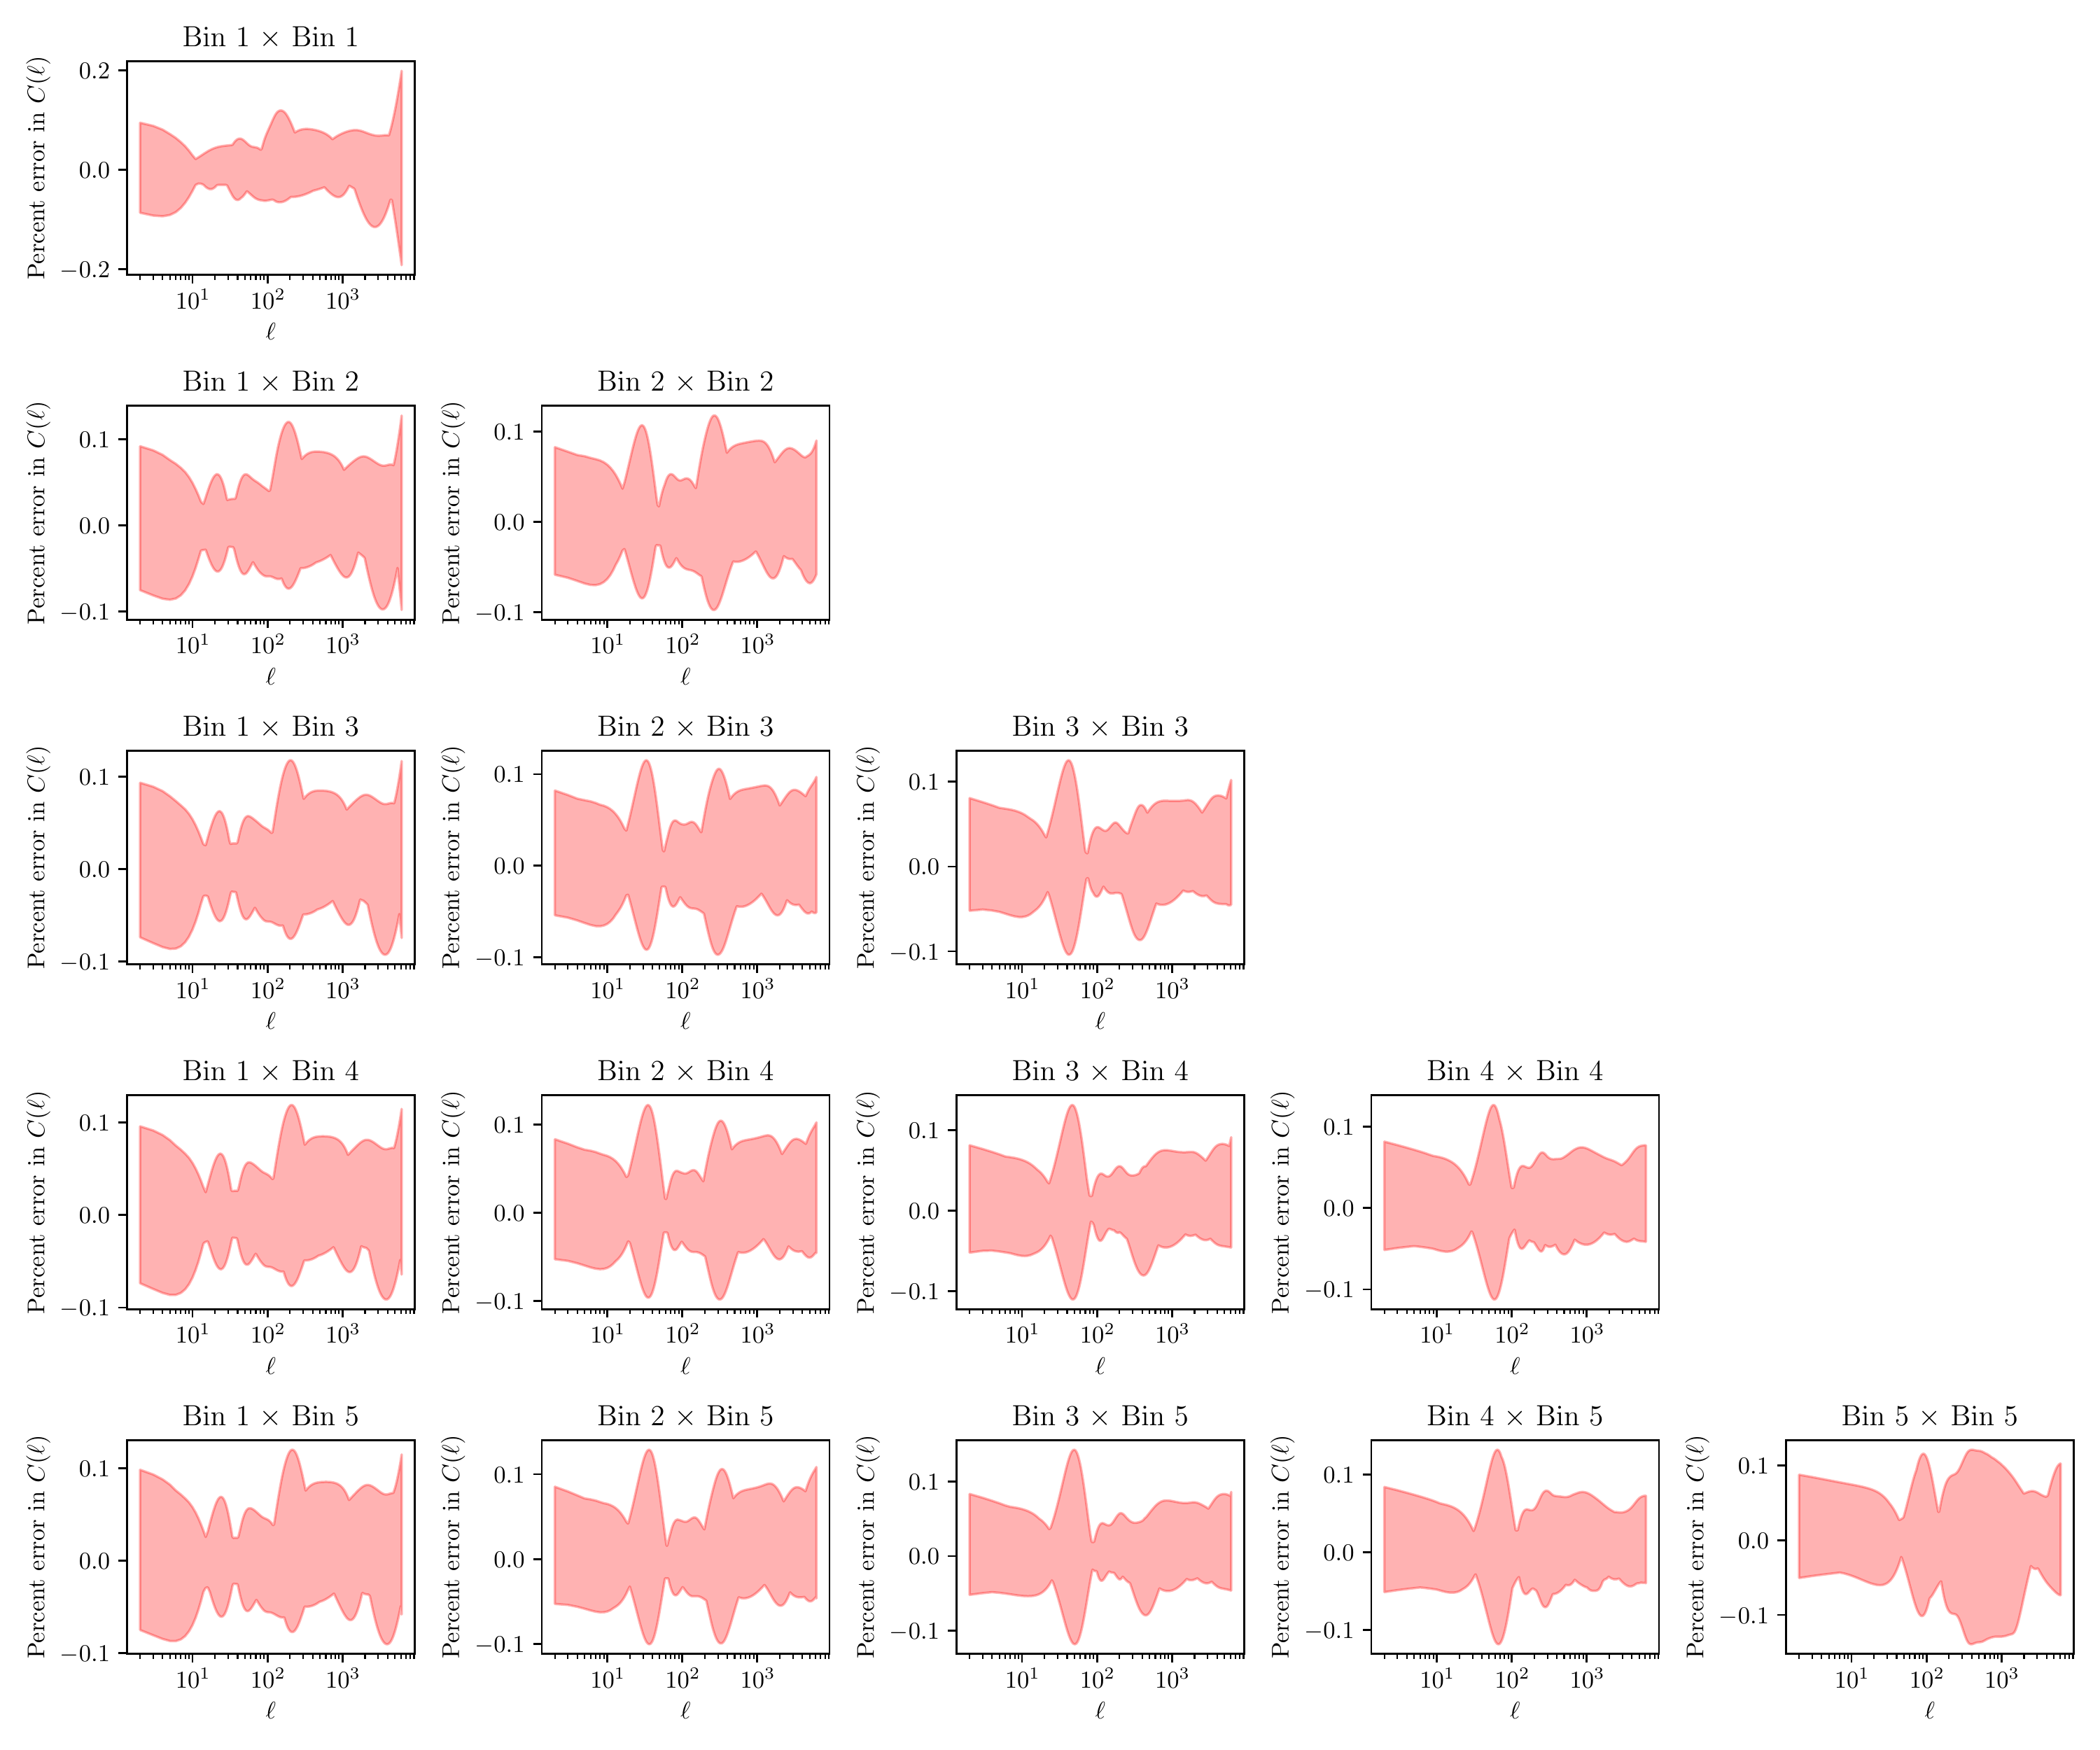}
%     \caption{Accuracy of $C(\ell)$ emulation. Different panels show the range of the maximum and the minimum value as a percent error on $C(\ell)$. As can be seen, the accuracy of the emulated $C(\ell)~\lesssim~0.2\%$.}
%     \label{fig:Cl_emu}
% \end{figure*}

% \begin{figure*}
%     \centering
%     \includegraphics[width=\linewidth]{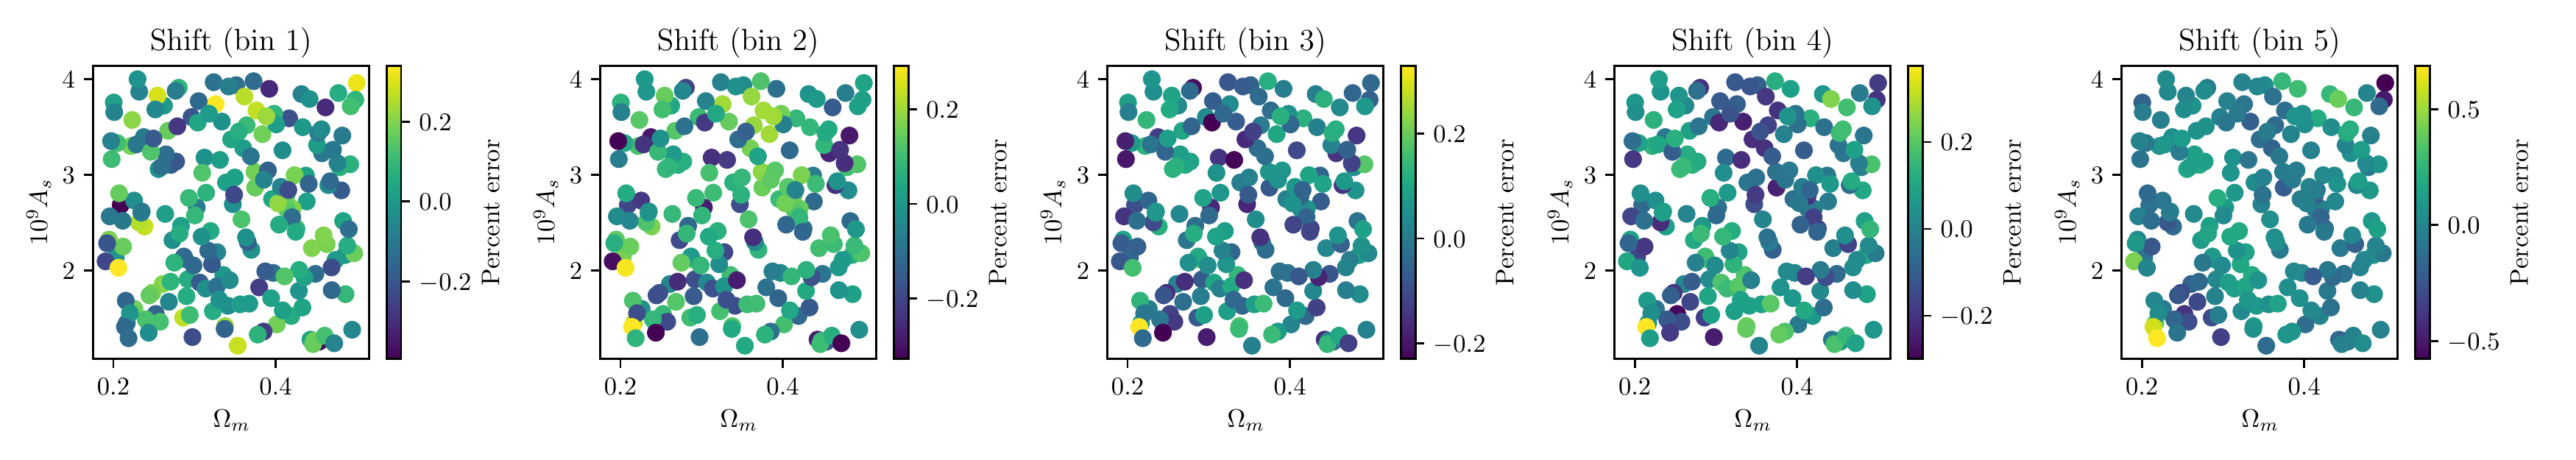}
%     \caption{Accuracy of the emulated shift parameters. We see that the emulated shift parameters are accurate to $\lesssim~0.5\%$.}
%     \label{fig:shift_emu}
% \end{figure*}

As mentioned in section \ref{ssec:cosmo_sampling}, we use a polynomial chaos expansion (PCE) emulator to calculate cosmological parameters dependent quantities such as the power spectrum and the shift parameters. Using the emulator leads to a manifold speedup of these calculation. However, in order to get unbiased results, we need to validate the accuracy of our emulator. 

In order to assess the accuracy of the emulator, we do a `leave-one out' test on our emulator. In this test, we leave one data point used in the full emulator training. By training the emulator on rest of the cosmological parameters, we predict the data vector at the left-out parameter. We then compare the predicted data vector to the `true' calculated data vector. Using such a leave out one test, we find that our emulator predicts the power spectrum at $\lesssim~0.2\%$. Note that this is much lower than the intrinsic uncertainty of the halofit \citep{Takahashi2012} power spectrum model. The uncertainty due to the emulator in the estimated auto and cross power spectrum is shown in Figure \ref{fig:Cl_emu}. Similarly, the emulated shift parameters are accurate to $\lesssim 0.5\%$ as shown in Figure \ref{fig:shift_emu}.
