# Supplementary material for: Map-based cosmology inference with lognormal cosmic shear maps
Source: arXiv:2204.13216 source file (2022-04-27)
Supplement: Supplementary file 2 [file sampling_efficiency.tex]

\section{Sampling efficiency}\label{sec:efficiency}

\begin{figure*}
    \centering
    \includegraphics[width=0.8\linewidth]{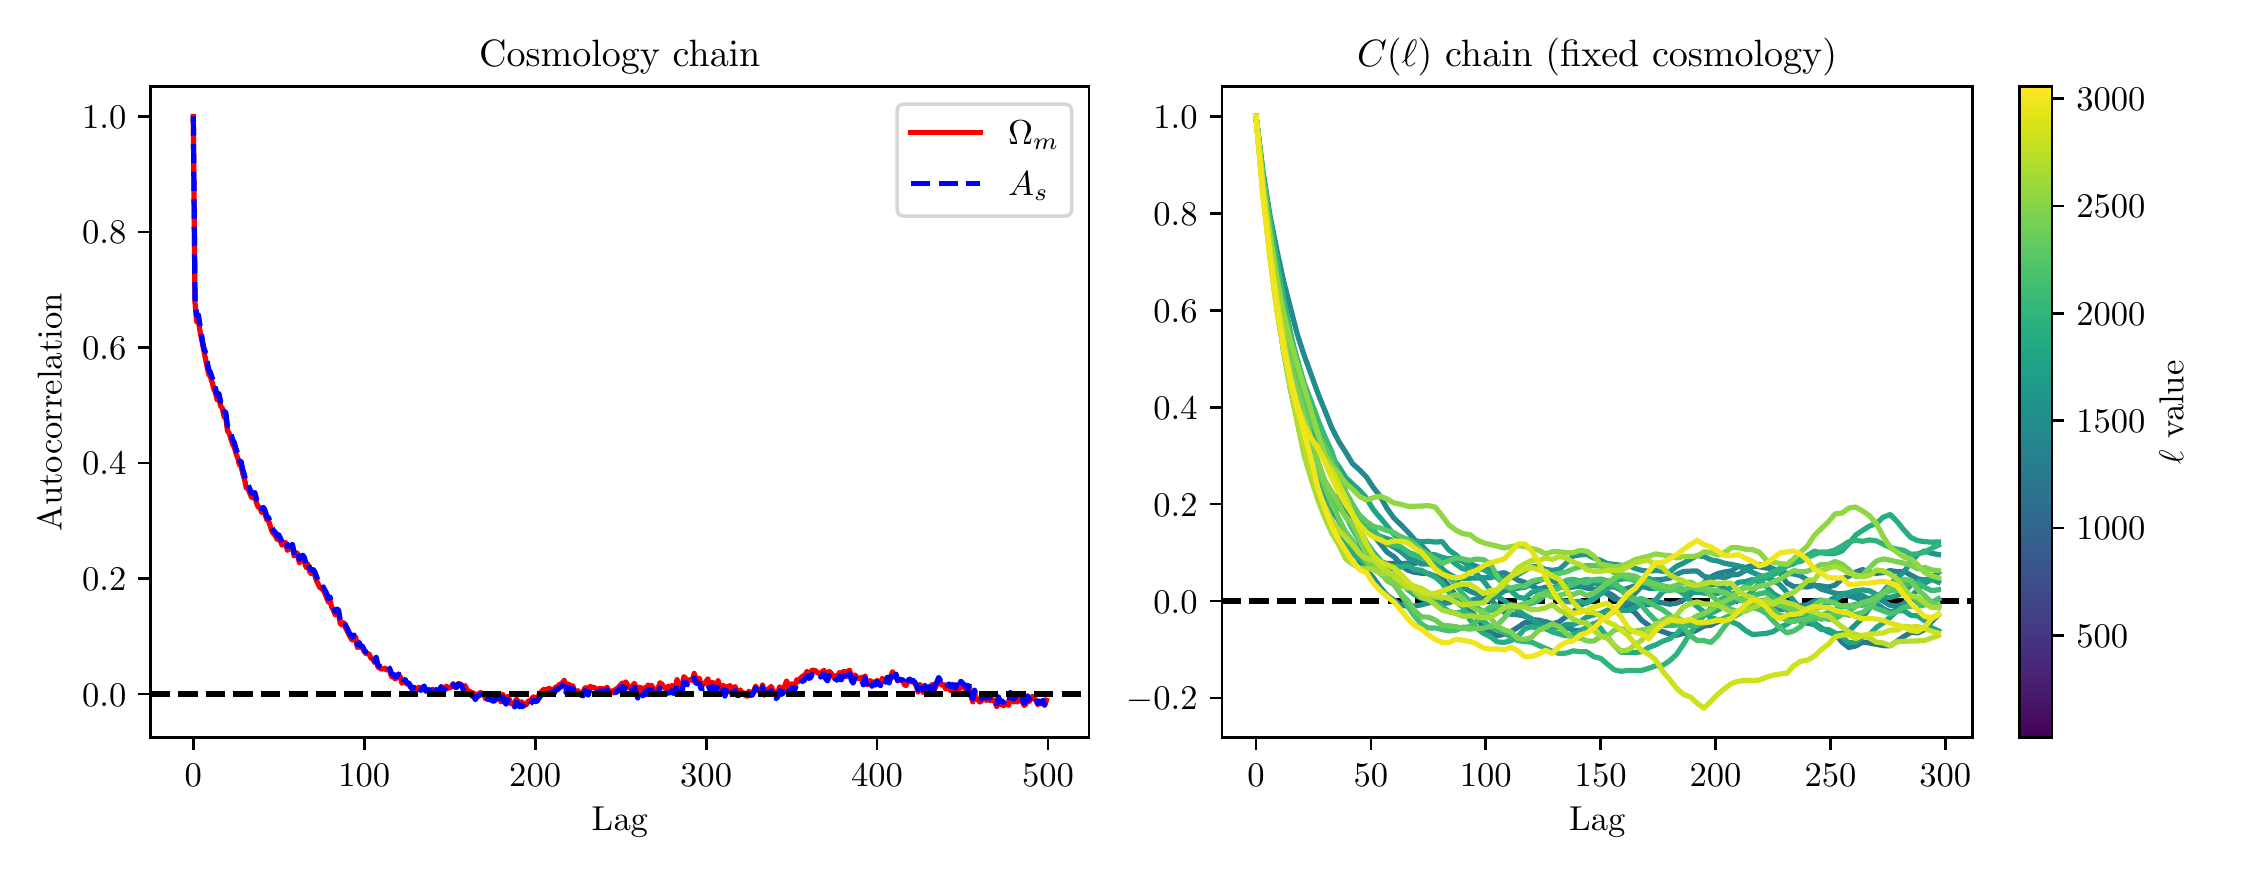}
    \caption{The autocorrelation of the MCMC chains. {\it (left)}: Autocorrelation of the cosmology chains in a run of our algorithm. {\it (right)} Autocorrelation of the $C(\ell)$ chains (angular power spectrum calculated for each map in the sample) with fixed cosmological parameters. The color shows the auto-correlation for $C(\ell)$ at different $\ell$ values. As can be seen from the figure, the correlation length of the chains are reasonably short to allow for simultaneous sampling of the mass maps and cosmological parameters. The integrated autocorrelation length of the cosmology chains are $< 100$, and the integrated autocorrelation length for the fixed cosmology $C(\ell)$ chains are $< 50$.
    } 
    \label{fig:autocorr}
\end{figure*}

A major problem for sampling based forward-modelled reconstruction methods is the long correlations in the HMC chains. Specifically, if the decorrelation length of the map sampling is large, then simultaneous sampling of the cosmological parameters can become numerically unfeasible.  We demonstrate here that this is not a problem in our implementation.

A necessary condition for being able to use our method to sample cosmological parameters is to have a reasonably short correlation length for the map samples with fixed cosmology. In the right panel of Figure \ref{fig:autocorr}, we show the correlation function of the power spectrum chain for a run of our code on a simulated dataset with fixed cosmological parameters. As can be seen in the Figure, we do not have an unresonably high correlation length, thus allowing for the simultaneous sampling of cosmological parameters. The integrated correlation length of the slowest modes is $< 50$.

We next look at the autocorrelation function for the cosmology chains when simultaneously sampling the cosmological parameters. We plot the autocorrelation for $\Omega_m$ and $A_s$ chains from our runs on the left panel of Figure \ref{fig:autocorr}. Our recovered correlation lengths are less than $100$. Given this short correlation length, we can use our code to simultaneously sample the mass maps as well as the cosmological parameters.
