# Supplementary material for: Map-based cosmology inference with lognormal cosmic shear maps
Source: arXiv:2204.13216 source file (2022-04-27)
Supplement: Supplementary file 3 [file LN_shift_calculation.tex]

\section{Lognormal shift calculation}\label{sec:ln_shift_calc}
