# Supplementary material for: Map-based cosmology inference with lognormal cosmic shear maps
Source: arXiv:2204.13216 source file (2022-04-27)
Supplement: Supplementary file 4 [file analytic_posterior.tex]

\section{Analytic posterior for Gaussian prior}\label{sec:analytic_posterior}
In section \ref{sec:results}, we showed that we can get a posterior on the cosmological parameters by sampling from the conditional posteriors in a block sampling scheme. For the case of Gaussian prior, the marginalization can be done analytically and therefore be compared with the sampling based posterior to validate the posteriors. In the rest of this section, we follow the notations of \citet{Jeffrey2018}. 

Using Bayes Theorem, we can write the posterior on the cosmological parameters, $\Theta$, as
\begin{equation}
    P(\Theta|\mD) \propto P(\mD|\Theta)P(\Theta),
\end{equation}
where, $P(\Theta)$ is the prior on the cosmological parameters. The likelihood term involves a marginalization over the convergence maps, $\mvec{\kappa}$ and can be written as, 
\begin{equation}\label{eqn:marginalized_likelihood}
    P(\mD | \Theta) = \int d\mvec{\kappa}~ P(\mD|\mvec{\kappa}) P(\mvec{\kappa}|\Theta).
\end{equation}
In the above equation, we have assumed that the data depends on $\Theta$ only through its dependence on $\mvec{\kappa}$. Assuming a Gaussian prior, we can write,
\begin{equation}\label{eqn:prior}
    P(\mvec{\kappa}|\Theta) = \frac{1}{\sqrt{\text{det}(2\pi \mmat{S}_{\kappa})}}\exp\bigg[-\frac{1}{2}\mvec{\kappa}^{\dag} \mmat{S}^{-1}_{\kappa} \mvec{\kappa}\bigg].
\end{equation}
Note that the variance, $\mmat{S}_{\kappa}$ depends on the cosmological parameters. However for brevity we do not explicitly show the dependence on $\Theta$. The shear field depends on the convergence field through the forward Kaiser-Squires transformation, equation \eqref{eqn:fwd_KS}. The discretized version of this transformation can be thought of as a matrix multiplication by the transformation matrix, $\mmat{A}$, which is written as,
\begin{equation}
    \mvec{\gamma} = \mmat{A}\mvec{\kappa}.
\end{equation}
Since the shear field is non-local, in real space, the matrix $\mvec{A}$ is dense. However, in the Fourier space, the transformation is diagonal. 
\begin{equation}
    \tilde{\mmat{A}}_{ij}(\mvec{k}) = \frac{l^2_{x,i} - l^2_{y,i} - 2 i l_{x,i}l_{y,i}}{l^2_{x,i} + l^2_{y,i}}\delta^{K}_{ij}.
\end{equation}
Assuming a Gaussian likelihood for the observed shear and noise variance, given by $\mmat{N}$, we get,
\begin{equation}\label{eqn:lkl}
    P(\mD|\mvec{\kappa}) = \frac{1}{\sqrt{\text{det} (2\pi\mmat{N})}}\exp\bigg[-\frac{1}{2}
    (\mvec{\gamma}_{\text{obs}} - \mmat{A} \mvec{\kappa})^{\dag}\mmat{N}^{-1} (\mvec{\gamma}_{\text{obs}} - \mmat{A} \mvec{\kappa}) \bigg]
\end{equation}
Combining equations \eqref{eqn:prior} and \eqref{eqn:lkl} in equation, \eqref{eqn:marginalized_likelihood}, we can write,
\begin{align}\label{eqn:analytic_posterior}
 P(D|\kappa) P(\kappa | \Theta) &\propto \nonumber \\ 
 \frac{1}{\sqrt{\text{det}(2\pi \mmat{S}_{\kappa}})} &\exp \bigg[-\frac{1}{2} (\mvec{\kappa} - \mvec{\kappa}_{\text{WF}})^{\dag} \mmat{S}^{-1}_{\text{WF}}(\mvec{\kappa} - \mvec{\kappa}_{\text{WF}})\bigg] \nonumber \\  &\exp\bigg[\frac{1}{2}\mvec{\kappa}^{\dag}_{\text{WF}}\mmat{S}^{-1}_{\text{WF}} \mvec{\kappa}_{\text{WF}}\bigg]
\end{align}
where, 
\begin{equation}
    \mmat{S}_{\text{WF}} = (\mmat{S}^{-1}_{\kappa} + \mmat{A} \mmat{N}^{-1}\mmat{A}^{\dag})^{-1},
\end{equation}
and, $\mvec{\kappa}_{\text{WF}}$ is the Wiener-filtered convergence field given by,
\begin{equation}
    \mvec{\kappa}_{\text{WF}} = \mmat{W} \mvec{\gamma}_{\text{obs}}.
\end{equation}
in the above equation, the Wiener filter, $\mmat{W}$ is given as,
\begin{equation}
    \mmat{W} = \mmat{S}_{\kappa} [\mmat{S}_{\kappa} + \mmat{A}^{\dag}\mmat{N}\mmat{A}]^{-1} \mmat{A}^{\dag}.
\end{equation}
With this simplification, we can analytically marginalize the convergence field in equation \eqref{eqn:analytic_posterior}, resulting in the following expression for the marginalized likelihood for the cosmological parameters,
\begin{equation}
    P(\mD | \Theta) \propto \sqrt{\frac{\text{det}(2\pi \mmat{S}_{\text{WF}})}{\text{det}(2\pi \mmat{S}_{\kappa})}} \exp\bigg[\frac{1}{2}\mvec{\kappa}^{\dag}_{\text{WF}}\mmat{S}^{-1}_{\text{WF}} \mvec{\kappa}_{\text{WF}}\bigg].
\end{equation}
Note that, to infer cosmological parameters using this expression, we need to do the Weiner Filtering for each cosmological parameters. in general, the Weiner filtering of the convergence field is not trivial. For a realistic survey, there is no basis in which both the $\mmat{S}_{\kappa}$ and $\mmat{N}$ are sparse. $\mmat{S}_{\kappa}$ is diagonal in the Fourier basis, while the noise covariance, $\mmat{N}$ is diagonal in the real basis. However, if we simplify by assuming that the number of galaxies in each pixel are the same, the noise covariance matrix is also diagonal in the Fourier basis and then we can do fast Weiner filtering of the convergence field. 

Note that the Kaiser-Squires inversion matrix, $\mmat{A}$ becomes non-hermitian for the Nyquist frequencies due to resolution effects. Therefore in order to compare the cosmological contours of our HMC code and the analytically-marginalized posterior, we mask the Nyquist frequencies in our simulations and in our inference. We compare our results for a LSST-like survey with a pixel resolution of $20$ arcminute. The resulting cosmological contours are shown in Figure \ref{fig:analytic_cosmo_contours}. As we can see from the Figure, the two contours are remarkably similar. Using the p

\begin{figure}
    \centering
    \includegraphics[width=\linewidth]{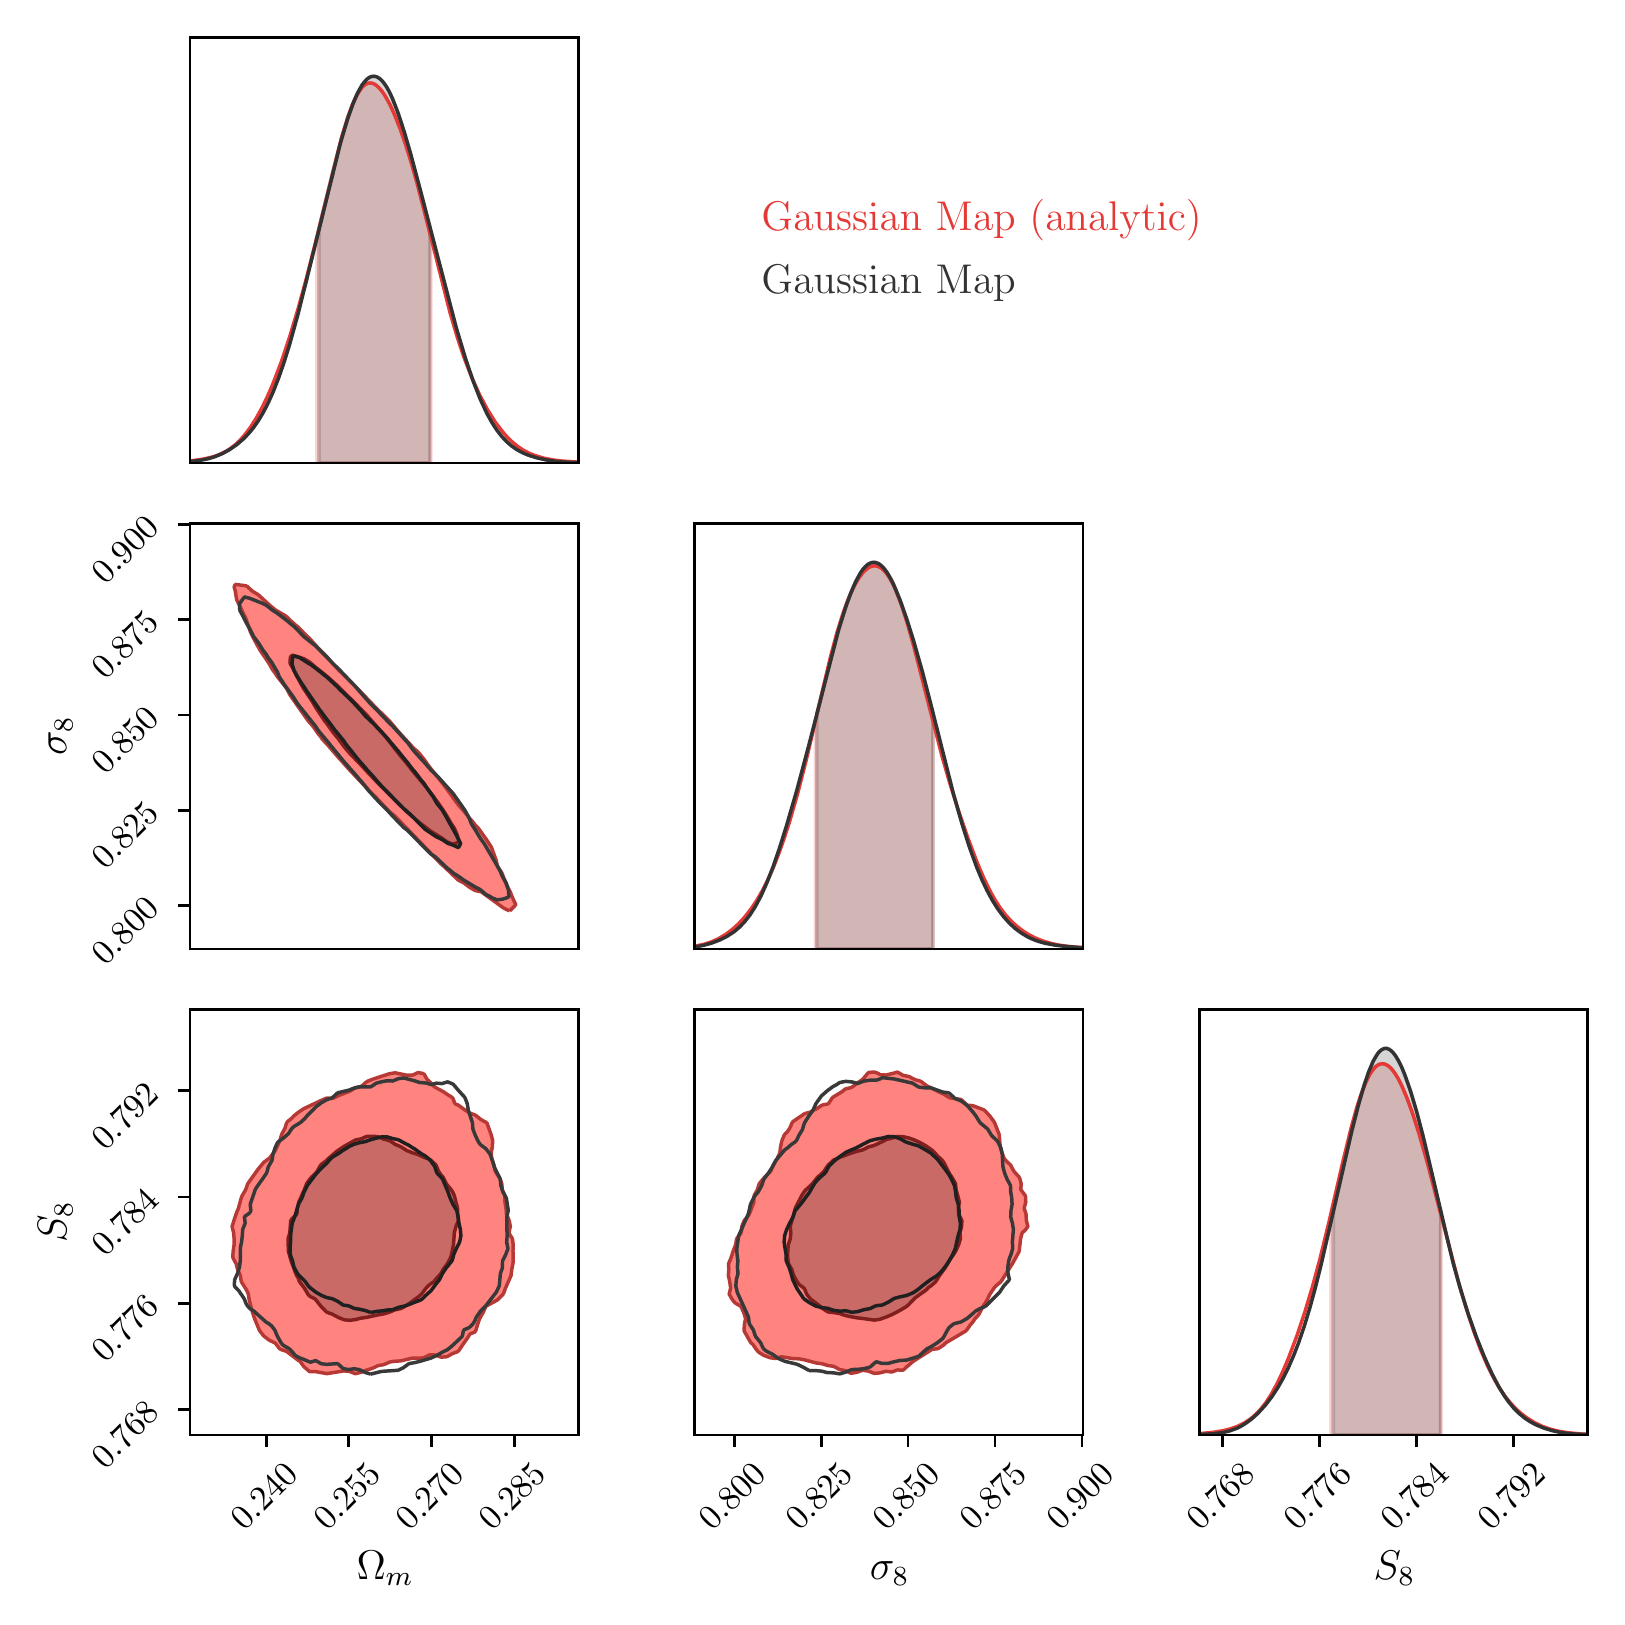}
    \caption{Comparison of the cosmology contours obtained from our map-based inference code and the analytic marginalization of the mass maps as described in section \ref{sec:analytic_posterior}. In this comparison, we mask the Nyquist frequencies as the KS matrix, $\mmat{A}$, for these frequencies are rendered non-Hermitian due to resolution effects. The resulting contours from the HMC code and the analytical marginalization based code are consistent with each other.}
    \label{fig:analytic_cosmo_contours}
\end{figure}
